# Supplementary material for: CrossCBR: Cross-view Contrastive Learning for Bundle Recommendation
Source: arXiv:2206.00242 source file (2023-01-15)
Supplement: Supplementary file 1 [file 7_appendix.tex]

\newpage
\appendix
\section{Appendix} \label{sec:app}
